# Supplementary material for: Measurement-Driven Transitions between Area Law Phases
Source: arXiv:2509.15634 source file (2025-09-19)
Supplement: Supplementary file 1 [file SM.tex]

\documentclass[aps,prb,onecolumn,superscriptaddress]{revtex4-2}
\usepackage{amssymb}
\usepackage{graphicx}
\usepackage{booktabs}
\usepackage{amsmath}
\usepackage{amsthm}
\usepackage{amsfonts}
\usepackage[T1]{fontenc}
\usepackage{array}
\usepackage{multirow}
\usepackage{color}
\usepackage{esint}
\usepackage{bm}
\definecolor{LinkColor}{rgb}{0.75,0.0,0.2}
\usepackage{bbm}
\usepackage{hyperref}
\hypersetup{
	pdfauthor={good guys},
	pdftitle={good title},
	colorlinks=true,
	citecolor=LinkColor,
	linkcolor=LinkColor,
	urlcolor=LinkColor,
}
\usepackage{babel}
\usepackage{titlesec}

\begin{document}
\begin{center}
\textbf{\large Supplemental Material for "Measurement-Driven Transitions between Area Law Phase"}
\end{center}

\begin{figure}[htbp]
\begin{center}
\includegraphics[scale=0.65]{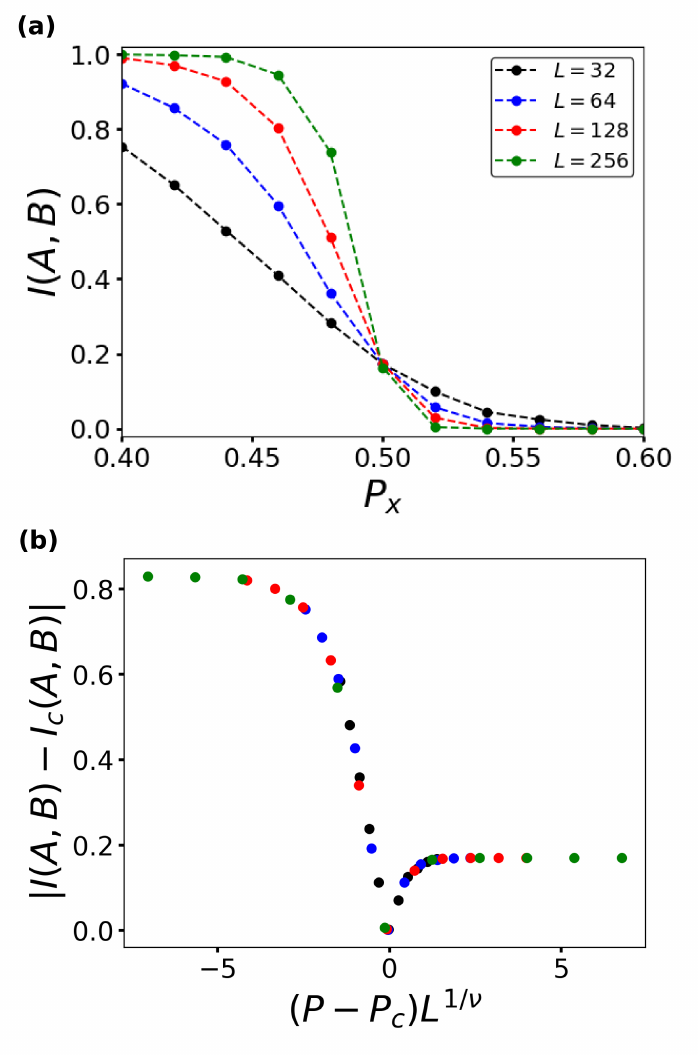}
\caption{\textbf{(a):} The mutual information $I(A,B)$ between two distant qubits versus the probability of single-qubit measurement $P_{X}$ with $P_{ZXZ}=0$. \textbf{(b):}  Scaling analysis of the data from the top panel. The data collapse occurs at the critical point $P_{c}=0.5$ and a critical exponent of $\nu=1.3$.}
\label{fig:CP Pzxz=0}
\end{center}
\end{figure}

\begin{figure}[htbp]
\begin{center}
\includegraphics[scale=0.65]{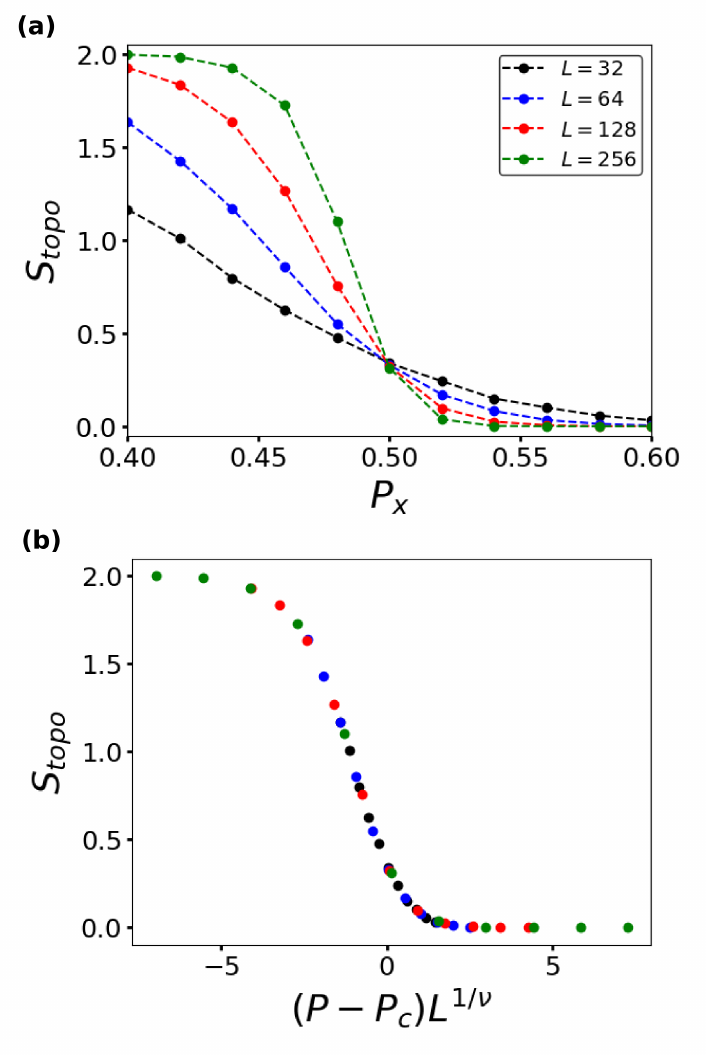}
\caption{\textbf{(a):} The topological entanglement entropy $S_{topo}$ versus the probability of single-qubit measurement $P_{X}$ with $P_{ZZ}=0$. \textbf{(b):}  Scaling analysis of the data from the top panel. The data collapse occurs at the critical point $P_{c}=0.5$ and a critical exponent of $\nu=1.3$.}
\label{fig:CP Pzz=0}
\end{center}
\end{figure}

\end{document}
